# Supplementary material for: Training Machine Learning Models to Characterize Temporal Evolution of Disadvantaged Communities
Source: arXiv:2303.03677 source file (2023-03-07)
Supplement: Supplementary file 1 [file appendix.tex]

\section{Model Parameters}
